# Supplementary material for: A Mathematical Exploration of Why Language Models Help Solve Downstream Tasks
Source: arXiv:2010.03648 source file (2021-04-14)
Supplement: Supplementary file 1 [file regression_appendix.tex]

\begin{table}[ht] % these results are in the downstream_tasks.ipynb notebook, clfs are saved by paths there
  \caption{Ratio of residual norm to the norm of $f^*$ for different datasets. A smaller value indicates a better fit, and 0 indicates a perfect fit.}
  \label{tab:reg_losses}
  \centering
  \begin{tabular}{lc}
    \toprule
    Task & Residual ratio \\
    \midrule
    DBPedia 	& 0.38 \\
    IMDb 		& 0.18 \\
    Yahoo 		& 1.72 \\
    TREC 		& 1.55 \\
    MPQA		& 1.28 \\
    CR			& 1.54 \\
    \bottomrule
  \end{tabular}
\end{table}
